# Supplementary material for: Temperature-tunable Fano resonance induced by strong coupling between Weyl fermions and phonons in TaAs
Source: arXiv:1608.08160 source file (2016-08-29)
Supplement: Supplementary file 1 [file SuppMat.pdf]

# Supplementary Information

# Temperature-tunable Fano resonance induced by strong coupling between Weyl fermions and phonons in TaAs

B. Xu[1,2,†], Y. M. Dai[3,†], L. X. Zhao[1], K. Wang[1], R. Yang[1], W. Zhang[1], J. Y. Liu[1], H. Xiao[2], G. F. Chen[1,4], S. A. Trugman[3,5], J.-X. Zhu[3,5], A. J. Taylor[6], D. A. Yarotski[3], R. P. Prasankumar[3,*], and X. G. Qiu[1,4,*]

[1]*Beijing National Laboratory for Condensed Matter Physics, Institute of Physics, Chinese Academy of Sciences, P.O. Box 603, Beijing 100190, China*

[2]*Center for High Pressure Science and Technology Advanced Research, Beijing 100094, China*

[3]*Center for Integrated Nanotechnologies, Los Alamos National Laboratory, Los Alamos, New Mexico 87545, USA*

[4]*Collaborative Innovation Center of Quantum Matter, Beijing 100190, China*

[5]*Theoretical Division, Los Alamos National Laboratory, Los Alamos, New Mexico 87545, USA*

[6]*Associate Directorate for Chemistry, Life and Earth Sciences, Los Alamos National Laboratory, Los Alamos, New Mexico 87545, USA*

[†]These authors contributed equally to this work.

[*]e-mail: rpprasan@lanl.gov; xgqiu@iphy.ac.cn

**Nature of the 253 cm$^{-1}$ mode** Non-centrosymmetric TaAs crystallizes in the $I4_1md$ space group (No. 109)[1,2] with the irreducible vibrational representation $[A_1 + E] + [A_1 + 2B_1 + 3E]$[3], where the first term represents acoustic modes and the second term corresponds to optical modes. While all the optical modes are Raman active, only the $A_1$ and $E$ modes are IR active. All of the optical phonons have been observed in a recent room-temperature Raman spectroscopy study[3]. The frequency (~253 cm$^{-1}$) of the phonon we observed in $R(\omega)$ agrees very well with the $A_1$ mode that was identified at ~252 cm$^{-1}$ by Raman spectroscopy. Furthermore, the $E$ modes involve vibrations in the $ab$ plane, while the $A_1$ mode arises from vibrations along the $c$ axis[3]. The absence of the 253 cm$^{-1}$ mode in $R(\omega)$ measured on the (001) surface, as shown in Fig. S2, indicates that it is active along the $c$ axis. These observations demonstrate that the 253 cm$^{-1}$ phonon in $R(\omega)$ is associated with the $A_1$ mode.

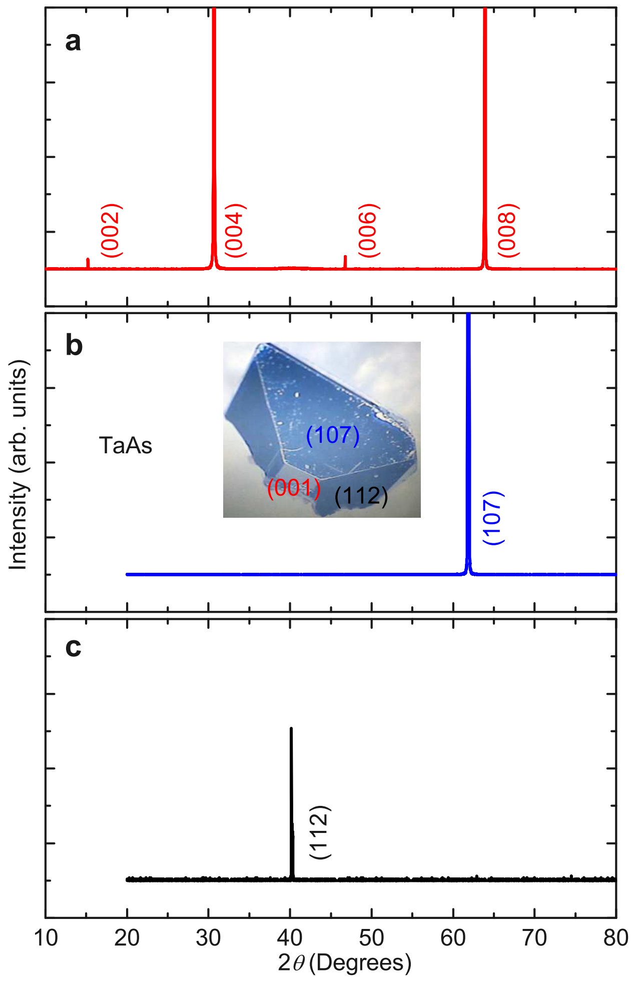


**Figure S1 | X-ray diffraction of TaAs. a–c**, X-ray diffraction patterns from the (001), (107) and (112) surfaces of an as-grown TaAs single crystal, respectively. The inset of **b** shows an optical image of the measured single crystal, where the Miller indices are marked on corresponding surfaces.

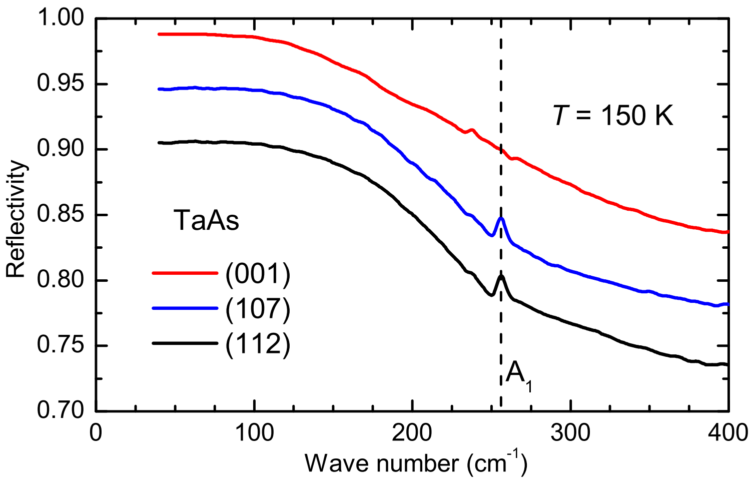


**Figure S2 | Far-infrared reflectivity of TaAs.** Reflectivity $R(\omega)$ in the far-infrared region measured at 150 K on three different surfaces of TaAs: (001) (red curve), (107) (blue curve), and (112) (black curve). The sharp peak at $\sim$253 cm$^{-1}$ in $R(\omega)$ measured on the (107) and (112) surfaces is associated with the IR-active $A_1$ mode. This mode is active along the $c$ axis, in good agreement with the fact that it is absent in the $R(\omega)$ spectrum measured on the (001) surface.

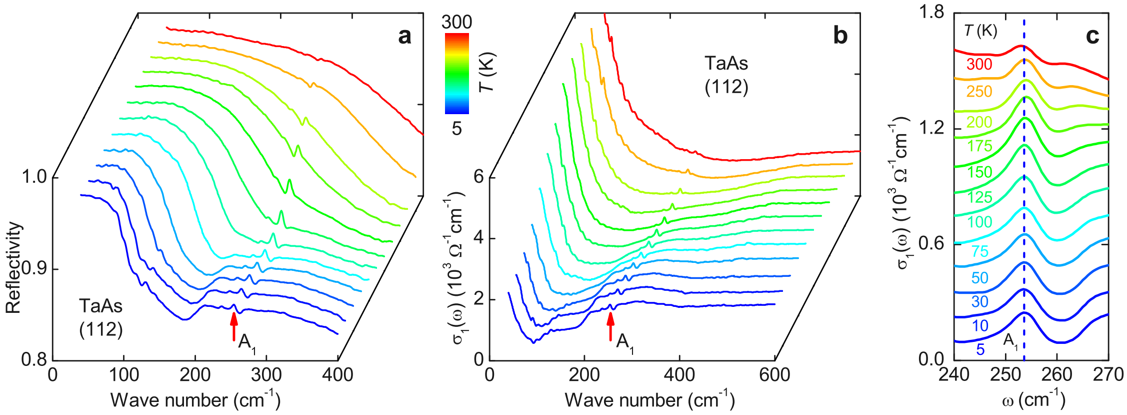


**Figure S3** | **Reflectivity and optical conductivity of TaAs.** **a**, Far-infrared $R(\omega)$ of TaAs measured on the (112) surface at 12 different temperatures from 5 to 300 K. **b**, Optical conductivity $\sigma_1(\omega)$ of TaAs on the (112) surface at different temperatures calculated from $R(\omega)$ using a Kramers-Kronig analysis. The sharp feature associated with the $A_1$ mode is indicated by a red arrow in both the $R(\omega)$ and $\sigma_1(\omega)$ spectra. **c**, Enlarged view of the optical conductivity in the frequency range of the IR-active $A_1$ mode. The line shape of this mode exhibits pronounced asymmetry at low temperatures, signaling strong electron-phonon coupling. The asymmetry of the phonon line shape varies dramatically with temperature. All of these observations are identical to the ones made on the (107) surface.

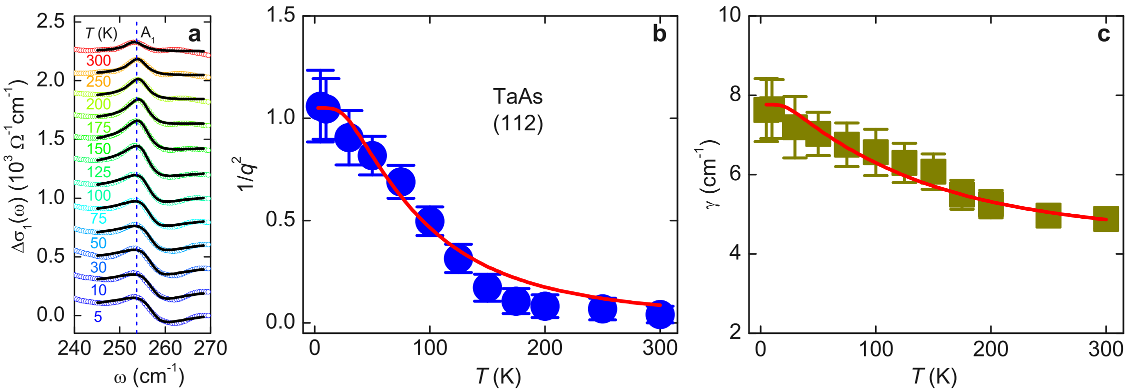


**Figure S4 | Fano fit to the phonon line shape and temperature dependence of the fitting parameters. a**, Line shape of the $A_1$ phonon, extracted from the optical conductivity measured at different temperatures on the (112) surface of TaAs. The black solid lines through the data represent the Fano fitting results. **b**, Temperature dependence of the Fano parameter $1/q^2$, which describes the asymmetry of the phonon line shape. The red solid curve is the least-square fit using Eq. (2) in the main text. **c**, The phonon linewidth $\gamma$ as a function of temperature. The red solid curve denotes the least-square fitting result using the summation of Eq. (4) and Eq. (5) in the main text.

# References


1. Weng, H., Fang, C., Fang, Z., Bernevig, B. A. & Dai, X. Weyl Semimetal Phase in Noncentrosymmetric Transition-Metal Monophosphides. *Phys. Rev. X* **5**, 011029 (2015).

2. Huang, S.-M. *et al.* A Weyl Fermion semimetal with surface Fermi arcs in the transition metal monopnictide TaAs class. *Nat. Commun.* **6**, 7373 (2015).

3. Liu, H. W. *et al.* Raman study of lattice dynamics in the Weyl semimetal TaAs. *Phys. Rev. B* **92**, 064302 (2015).
